# Supplementary material for: RepQ: Generalizing Quantization-Aware Training for Re-Parametrized Architectures
Source: arXiv:2311.05317 source file (2023-11-09)
Supplement: Supplementary file 2 [file supp_acronyms.tex]

\DeclareAcronym{nn}{
    short = NN,
    long = Neural Networks,
}

\DeclareAcronym{qat}{
    short = QAT,
    long = Quantization\-/Aware Training,
}

\DeclareAcronym{bn}{
    short = BN,
    long = Batch Normalization,
}

\DeclareAcronym{fp}{
    short = FP,
    long = Floating-Point
}

\DeclareAcronym{lr}{
    short = LR,
    long = Learning Rate
}
